# Supplementary material for: Dancing Between Success and Failure: Edit-level Simplification Evaluation using SALSA
Source: arXiv:2305.14458 source file (2023-10-22)
Supplement: Supplementary file 1 [file typology.tex]

\begin{figure*}[ht!]
    \centering
    \includegraphics[width=0.99\textwidth]{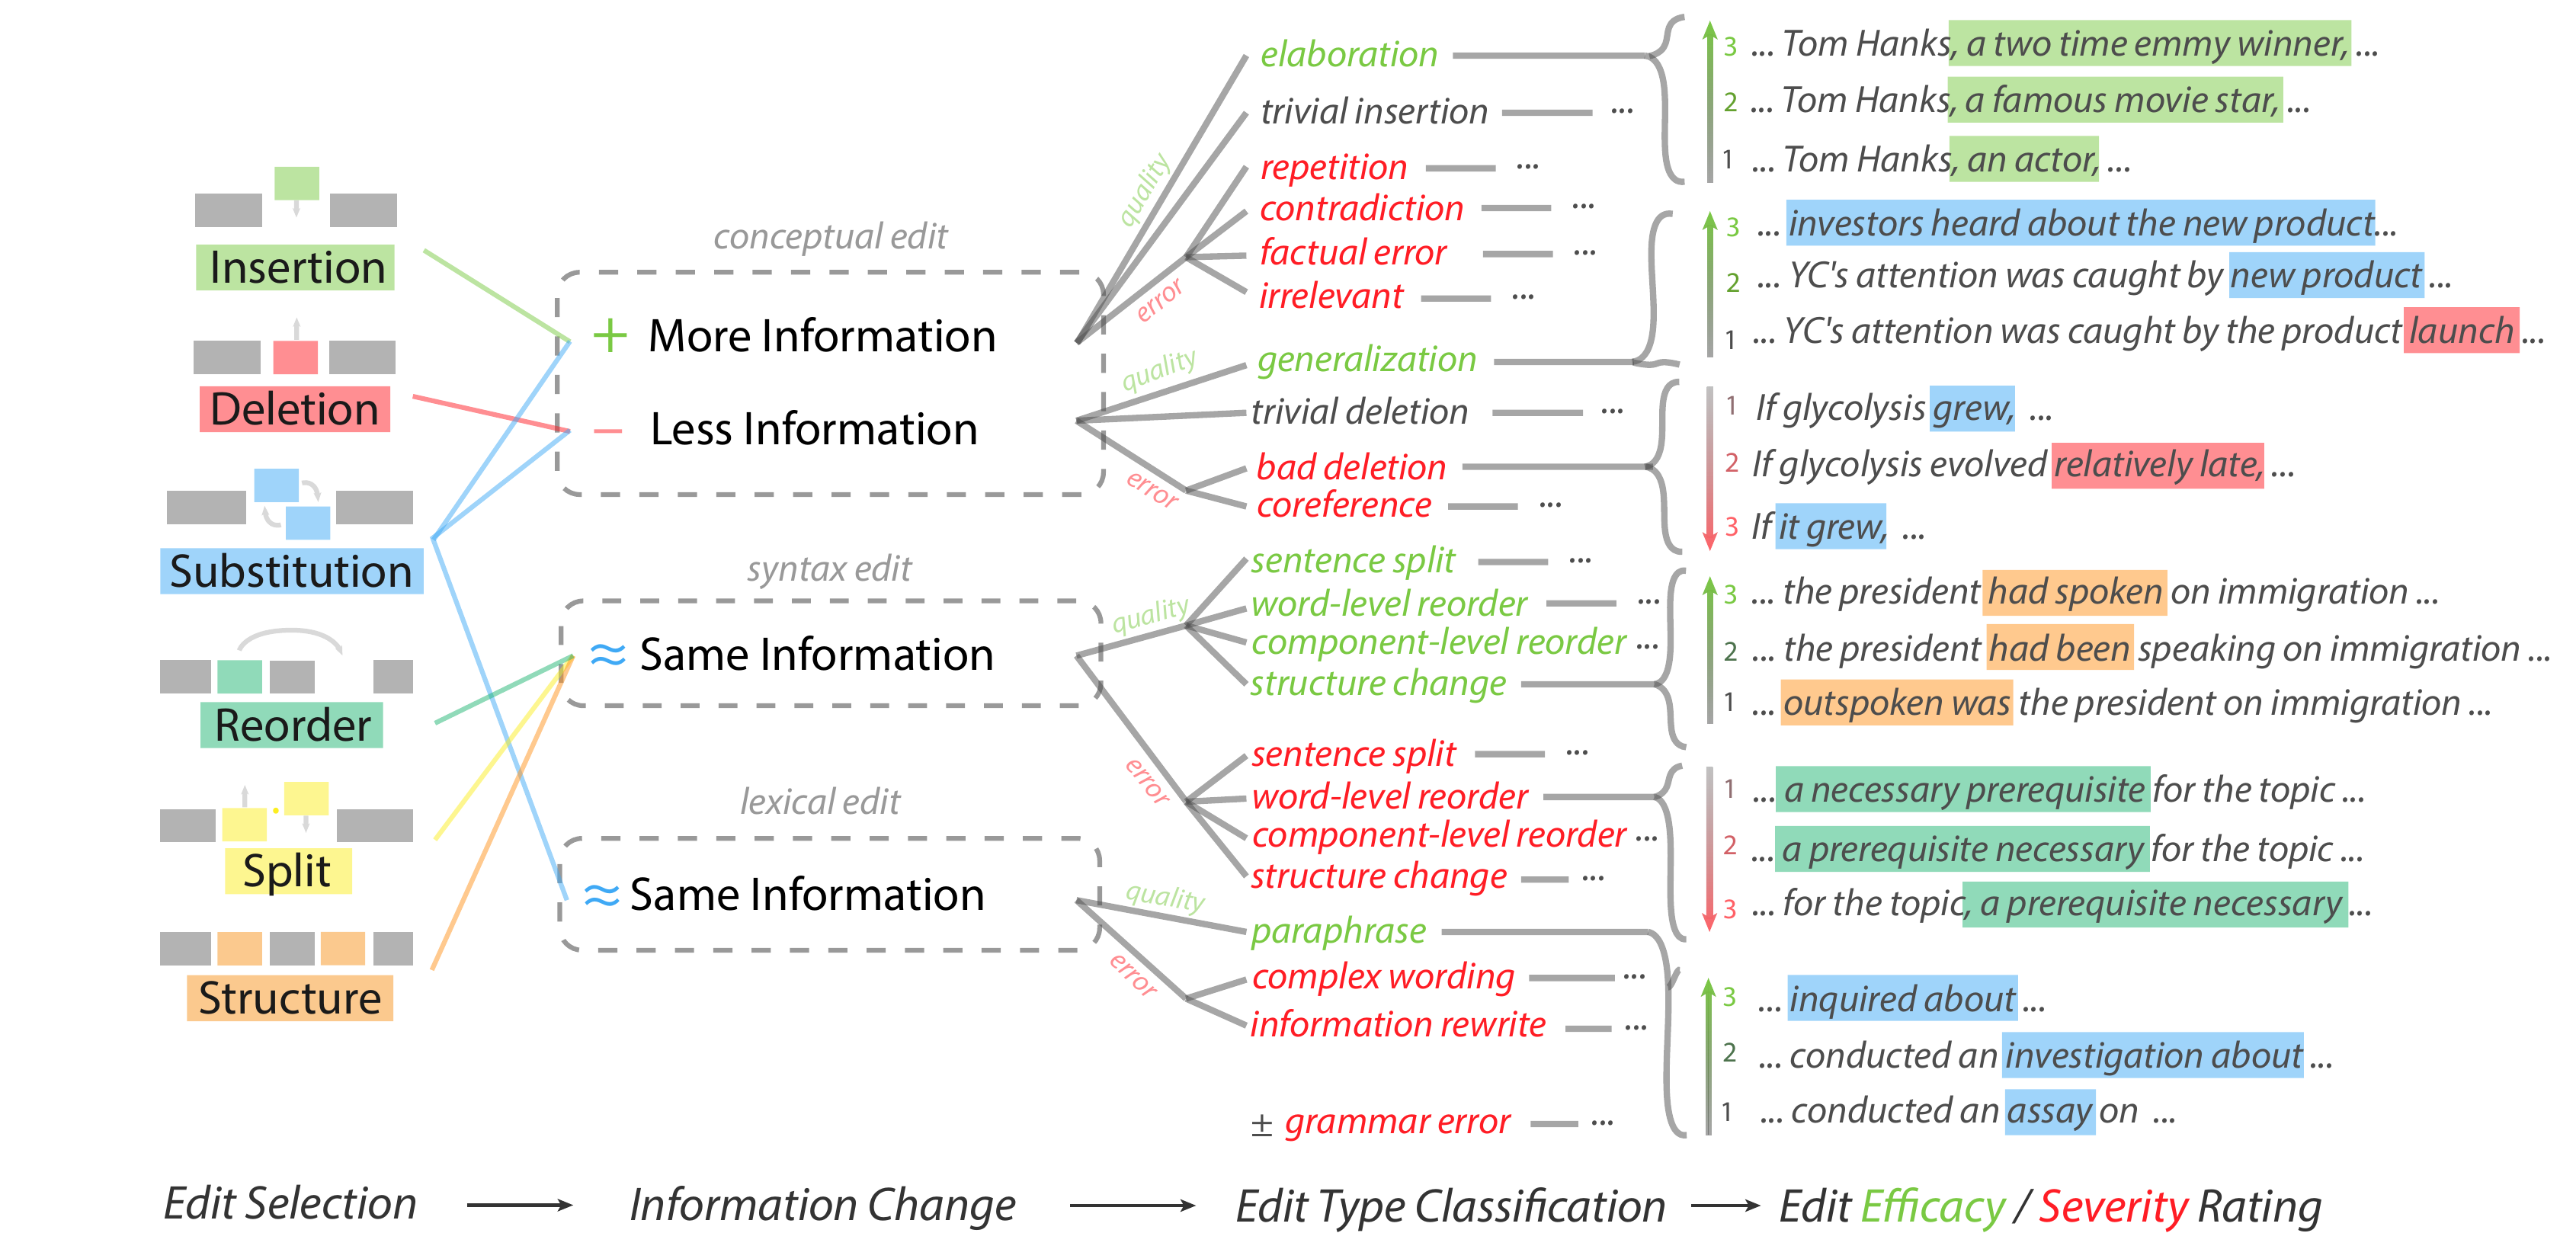}
    \setlength{\belowcaptionskip}{-10pt}
    \captionof{figure}{The multi-stage \framework{} edit evaluation framework, implemented by our edit annotation interface (Fig. \ref{fig:annotation-scheme}). Underlying spans are classified into twenty one {\color{limegreen} success} (↑) and {\color{red} failure} (↓) types, rated by efficacy or error severity.}
    \label{fig:decision-tree}
\end{figure*}
