# Supplementary material for: Dancing Between Success and Failure: Edit-level Simplification Evaluation using SALSA
Source: arXiv:2305.14458 source file (2023-10-22)
Supplement: Supplementary file 2 [file edit_weights.tex]

\setlength{\tabcolsep}{3pt}
\begin{table}[h!]
\centering
\resizebox{\columnwidth}{!}{
\begin{tabular}{lcc}
\toprule
\textbf{Edit Family} & \textbf{Quality Weight} & \textbf{Error Weight} \\ 
\midrule
 Conceptual Simplification & 3.5 & -1 \\
 Syntactic Simplification & 3 & -5 \\
 Lexical Simplification & 4.8 & -1\\
\bottomrule
\end{tabular}
}
\setlength{\belowcaptionskip}{-10pt}
\caption{Edit weighting $w(e)$ for sentence-level \framework{} score, fit to maximize agreement on \simpevaltt{} human ratings.}
\label{table:edit_weighting}
\end{table}
